# Supplementary material for: Analysis of Age of Information in Non-terrestrial Networks
Source: arXiv:2310.03969 source file (2023-10-06)
Supplement: Supplementary file 1 [file 0X_Appendix.tex]

\begin{appendix}
\subsection{Proof of Lemma 1} \label{pro:Lem1}

Based on the definition of $\mathrm{P}_{\mathrm{f}|\mathrm{f}}$, we make the assumption that an update is in the first off period at $t = 0$. To represent the start times of the $i$-th on- and off-service periods, we use $s'_i$ and $s_i$ respectively. As each on- and off-service period is distinct and non-overlapping, the probability of the next update remaining in an off-service period is obtained by summing the probabilities of arrival within each individual off-service period:
\begin{equation}
\begin{aligned} 
& \mathrm{P_{\mathrm{f}|\mathrm{f}}^{\mathrm{Cond}}} \\
    & \quad= \textstyle\sum_{i=1}^{\infty}F\left(s'_i\right)-F\left(s_i\right),\\
    & \quad= \textstyle\sum_{i=1}^{\infty}\exp\left(-\mu s_i\right)-\exp\left(-\mu\left(s_i+T_{f,i}\right)\right),\\
    & \quad= \textstyle\sum_{i=1}^{\infty}\left[1-\exp\left(-\mu T_{f,i}\right)\right]\textstyle \prod_{k=1}^{i-1}\exp\left(-\mu\left(T_{f,k}+T_{o,k}\right)\right).
\end{aligned}
\end{equation}
Further, we obtain that
\begin{equation}
\begin{aligned}
\mathrm{P_{\mathrm{f}|\mathrm{f}}} & =\textstyle\sum_{i=1}^{\infty}\mathbb{E}_{T_f}\left[1-e^{-\mu T_f}\right]\left(\mathbb{E}_{T_f}\left[e^{-\mu T_o}\right]\mathbb{E}_{T_o}\left[e^{-\mu T_f}\right]\right)^{i-1},\\
    & = \left(1-\frac{ \lambda_{ \mathrm{os} }}{\mu+ \lambda_{ \mathrm{os} }}\right)\sum_{l=0}^{\infty}\left(\frac{ \lambda_{ \mathrm{os} }}{\mu+ \lambda_{ \mathrm{os} }}\int e^{-\mu s}f_W(s)ds\right)^l,\\
    & = \frac{1-\frac{ \lambda_{ \mathrm{os} }}{\mu+ \lambda_{ \mathrm{os} }}}{1-\frac{ \lambda_{ \mathrm{os} }}{\mu+ \lambda_{ \mathrm{os} }}\int e^{-\mu s}f_W(s)ds}.
\end{aligned}
\end{equation}
Let $\mathrm{P}_\mathrm{off}$ denote the probability that a random point is in an off-service period. We have that
\begin{align}
    \mathrm{P}_\mathrm{off} &= \frac{\sum_{l=0}^{\infty}\mathbb{E}[T_{f,l}]}{\sum_{l=0}^{\infty}(\mathbb{E}[T_{f,l}]+\mathbb{E}[T_{o,l}])} = \frac{1}{1+ \lambda_{ \mathrm{o} }\mathbb{E}[W]}
\end{align}
and we obtain $\mathrm{P_{\mathrm{f}\mathrm{f}}} = \mathrm{P_{\mathrm{f}|\mathrm{f}}}\,\mathrm{P}_\mathrm{off}$ and $\mathrm{P_{\mathrm{f}\mathrm{o}}} = (1-\mathrm{P_{\mathrm{f}|\mathrm{f}}})\,\mathrm{P}_\mathrm{off}$. 
Since $\mathrm{P_{\mathrm{f}\mathrm{o}}} = \mathrm{P_{\mathrm{o}\mathrm{f}}}$, we have that
\begin{equation}
    \mathrm{P_{\mathrm{o}\mathrm{o}}} = 1 - \mathrm{P_{\mathrm{o}\mathrm{f}}} - \mathrm{P_{\mathrm{f}\mathrm{o}}} - \mathrm{P_{\mathrm{f}\mathrm{f}}} = 1-(2-\mathrm{P_{\mathrm{f}|\mathrm{f}}})\mathrm{P}_\mathrm{off}
\end{equation}
and obtain
\begin{align}
    \mathrm{P_{\mathrm{o}|\mathrm{o}}} = \frac{\mathrm{P_{\mathrm{o}\mathrm{o}}}}{1-\mathrm{P}_\mathrm{off}}.
\end{align}

\subsection{Proof of Lemma 2} \label{pro:Lem2}
Let $Z$ represent the interval time between two consecutive arrivals. Each arrival can be categorized into two situations: being accepted during the on-service period or being dismissed during the off-service period. After a dismissal, the system waits until a new arrival falls within the on-service period. Assuming that the subsequent arrival occurs during the on-service period when the previous one is accepted, we can easily derive
\begin{equation}
    \mathbb{E}\left[Y_{k}^{o}\right] = \mathbb{E}\left[Z\right] = \frac{1}{\mu}.
\end{equation}
Similarly, we obtain that
\begin{equation}
\begin{aligned}
    \mathbb{E}\left[Y_{k}^{f}\right] &= \sum_{n=2}^{\infty}\left[\sum_{l=1}^{n}\mathbb{E}\left[Z_l\right]\right]\mathrm{P_{\mathrm{f}|\mathrm{f}}}^{n-2}\left(1-\mathrm{P_{\mathrm{f}|\mathrm{f}}}\right),\\
    &= \frac{1}{\mu}\left(1+\frac{1}{1-\mathrm{P_{\mathrm{f}|\mathrm{f}}}}\right).
\end{aligned}
\end{equation}
The mean of $Y_k$ it thus given by
\begin{equation}
\mathbb{E}\left[Y_{k}\right]=\mathbb{E}\left[Y_{k}^{o}\right]\mathrm{P_{\mathrm{o}|\mathrm{o}}}+\mathbb{E}\left[Y_{k}^{f}\right](1-\mathrm{P_{\mathrm{o}|\mathrm{o}}}).
\end{equation}

Further, we can obtain the two terms forming the second moment of $Y_k$ respectively as
\begin{align}
    \mathbb{E}\left[Y_{k}^{2,o}\right] = \mathbb{E}\left[Z^2\right] = \frac{2}{\mu^2}
\end{align}
and
\begin{equation}
    \mathbb{E}\left[Y_{k}^{2,f}\right] = \sum_{n=2}^{\infty}\left[\left(\sum_{l=1}^{n}\mathbb{E}\left[Z_l\right]\right)^2\right]\mathrm{P_{\mathrm{f}|\mathrm{f}}}^{n-2}\left(1-\mathrm{P_{\mathrm{f}|\mathrm{f}}}\right).
\end{equation}
Since $Z_l$ follows exponential distribution with parameter $\mu$, we have $S_n = \textstyle\sum_{l=1}^{\infty}Z_l \thicksim \Gamma(n,\mu^{-1})$ and we obtain
\begin{equation}
\begin{aligned}
    \mathbb{E}\left[Y_{k}^{2,f}\right] &= \sum_{n=2}^{\infty}\left[\frac{n(n+1)}{\mu^2}\right]\mathrm{P_{\mathrm{f}|\mathrm{f}}}^{n-2}\left(1-\mathrm{P_{\mathrm{f}|\mathrm{f}}}\right),\\
    &= \frac{2}{\lambda^2}\frac{\mathrm{P_{\mathrm{f}|\mathrm{f}}^2}-3\mathrm{P_{\mathrm{f}|\mathrm{f}}}+3}{(1-\mathrm{P_{\mathrm{f}|\mathrm{f}}})^2}.
\end{aligned}
\end{equation}
The second moment of $Y_k$ thus yields
\begin{equation}
\mathbb{E}\left[Y_{k}^{2}\right]=\mathbb{E}\left[Y_{k}^{2,o}\right]\mathrm{P_{\mathrm{o}|\mathrm{o}}}+\mathbb{E}\left[Y_{k}^{2,f}\right](1-\mathrm{P_{\mathrm{o}|\mathrm{o}})}.
\end{equation}

\end{appendix}
